# Supplementary material for: Let-It-Flow: Simultaneous Optimization of 3D Flow and Object Clustering
Source: arXiv:2404.08363 source file (2024-08-13)
Supplement: Supplementary file 1 [file 6_supplementary.tex]

\section{Datasets and Code Implementation}

For datasets splits in comparison with MBNSFP~\cite{vidanapathirana2023mbnsf}, we maintain the philosophy of the aforementioned method and extract first frames from each sequence of Argoverse~\cite{Argoverse} and Waymo~\cite{Sun_2020_CVPR}.
For the main experiments against~\cite{Chodosh2023reevaluating,li2021neural,vidanapathirana2023mbnsf}, we extract the third frame from each Argoverse2~\cite{Argoverse} sequence, as we perform spatio-temporal clustering and past frames are always available. That resembles 150 unique scenes with various agents, motion and ego manuevers including rotational movement. We apply KISS-ICP~\cite{vizzo2023ral} on the sequences to compensate ego-motion for all methods. 

We used implementation of Chodosh~\cite{Chodosh2023reevaluating} from \url{https://github.com/kylevedder/zeroflow}, as it comes from the same group and no other official implementation is available. For MBNSFP~\cite{vidanapathirana2023mbnsf}, we used the official implementation from \url{https://github.com/kavisha725/MBNSF/tree/main}.

Our implementation is available on \url{https://github.com/vacany/let-it-flow}

% \section{Illustration of methods on dynamic objects}
